# Supplementary material for: Tracking perovskite crystallization via deep learning-based feature detection on 2D X-ray scattering data
Source: arXiv:2202.10983 source file (2022-02-22)
Supplement: Supplementary file 1 [file Supplementary-materials-Starostin-et-al-arXiv.pdf]

# Supplementary materials

## Tracking perovskite crystallization via deep learning-based feature detection on 2D X-ray scattering data

V. Starostin, V. Munteanu, A. Greco, E. Kneschaurek, A. Pleli, F. Bertram, A. Gerlach, A. Hinderhofer, and F. Schreiber

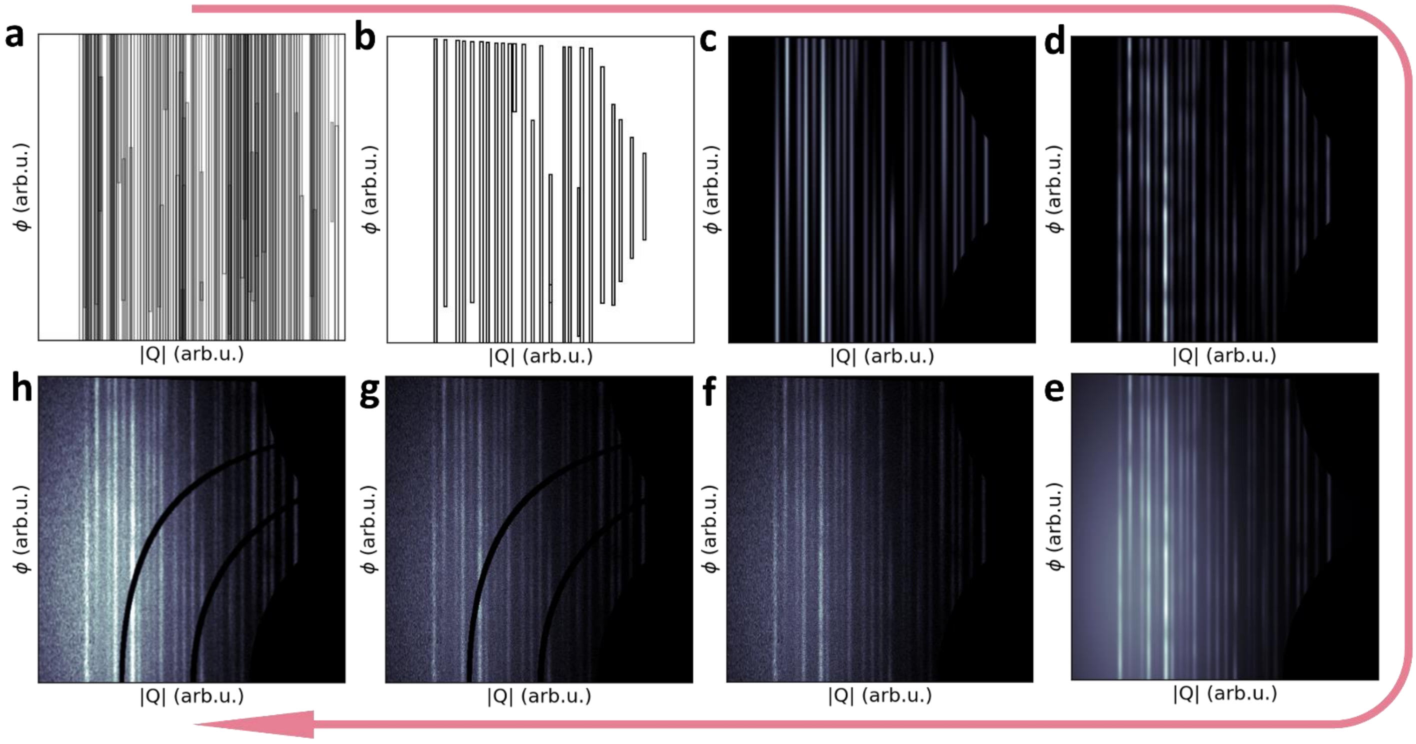


**Supplementary Figure 1** Simulation steps for the training data. (**a**) Generate peak characteristics (positions, sizes, intensities). (**b**) Filter out peaks in the dark areas and remove strong overlaps. (**c**) Generate Gaussian profiles corresponding to the peaks. (**d**) Modulate angular intensity distributions with Perlin noise. (**e**) Add scattering backgrounds. (**f**) Apply noise (Poisson, speckle noise, image digitalization). (**g**) Simulate detector gaps (curved in polar space) and geometry-determined dark areas. (**h**) Final simulation result (smoothing, contrast correction).

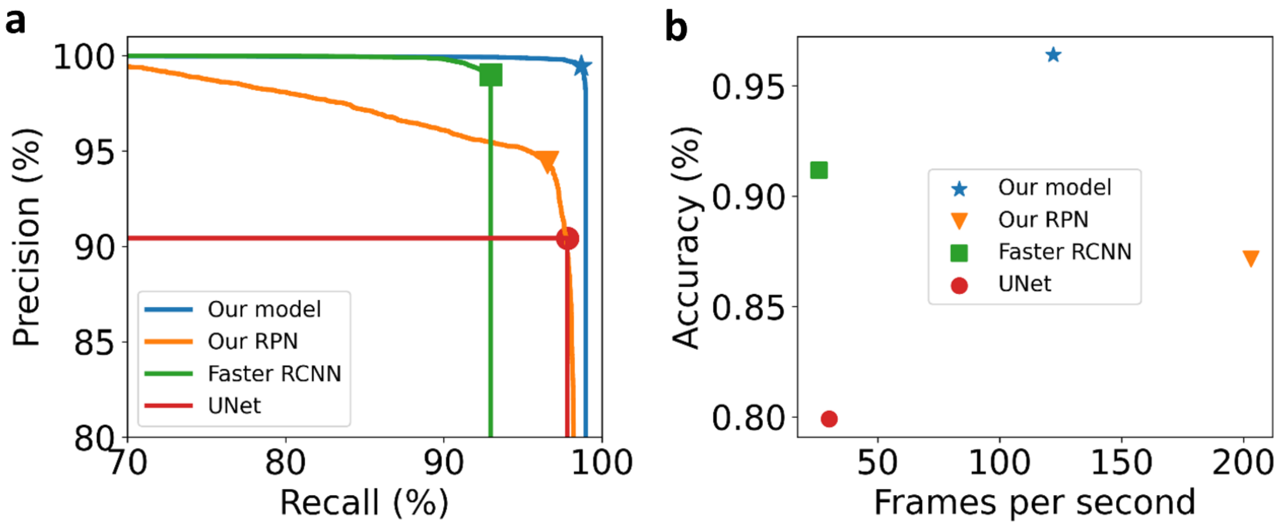


**Supplementary Figure 2** Detection performance metrics on the simulated data for our two-stage model, our Region Proposal Network (one-stage detector), the standard Faster R-CNN with ResNet-50 feature extractor and Feature Pyramid Network, and the U-Net model. (**a**) Precision-recall curves for different models obtained by varying level of confidence score and calculating the standard object detection metrics:

$\text{Recall} = \frac{matched\ peaks}{matched + missed\ peaks}$, $\text{precision} = \frac{matched\ peaks}{matched + false\ positives}$, $\text{accuracy} = \frac{matched\ peaks}{matched + missed + false\ positives}$. Markers denote the best detection accuracies on the test set for the studied models.

(**b**) Detection accuracies and speed (frames per second) for the compared models. The presented two-stage detector is the most accurate among the considered solutions and is sufficiently fast for real-time GIXD analysis.

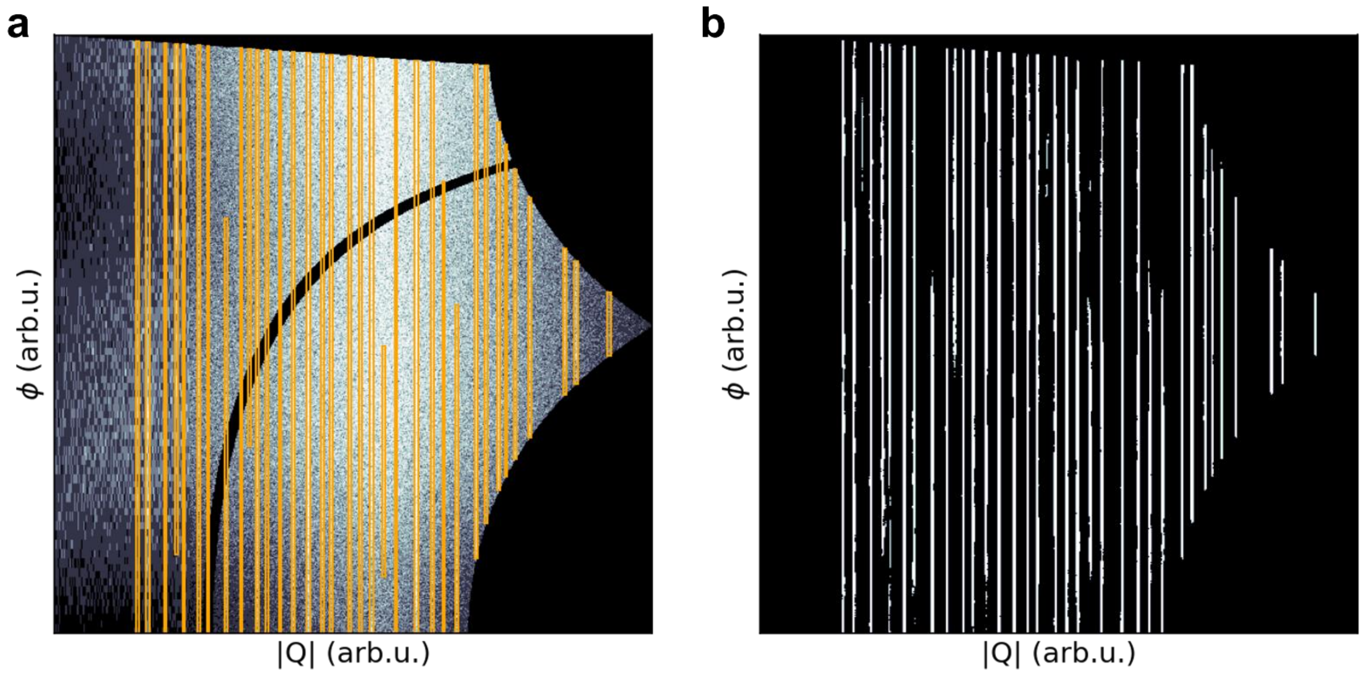


**Supplementary Figure 3** An example of the U-Net binary segmentation map (**b**) for a simulated GIXD image (**a**) with the ground truth peak positions illustrated by orange boxes. The black pixels on the segmentation map (**b**) correspond to the background and the white pixels correspond to the detected peaks. Apart from obvious false positive predictions, converting the segmentation map to the separated peak positions introduces additional errors. Such errors occur if a single peak results in multiple nonconnected segmentation areas, or if segmentation areas for several peaks are connected.

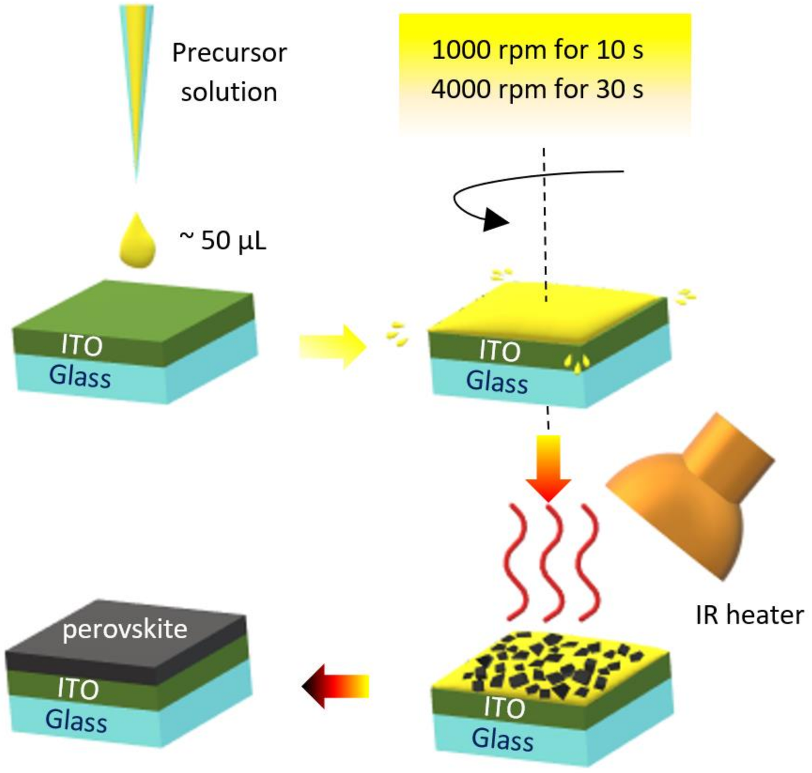


**Supplementary Figure 4** Thin perovskite film deposition procedure. 50 µL of precursor solution was spin-coated in 2 stages, 1000 rpm for 10 s and 4000 rpm for 30 s, and subsequently annealed by the IR heater, resulting in a dense perovskite film.

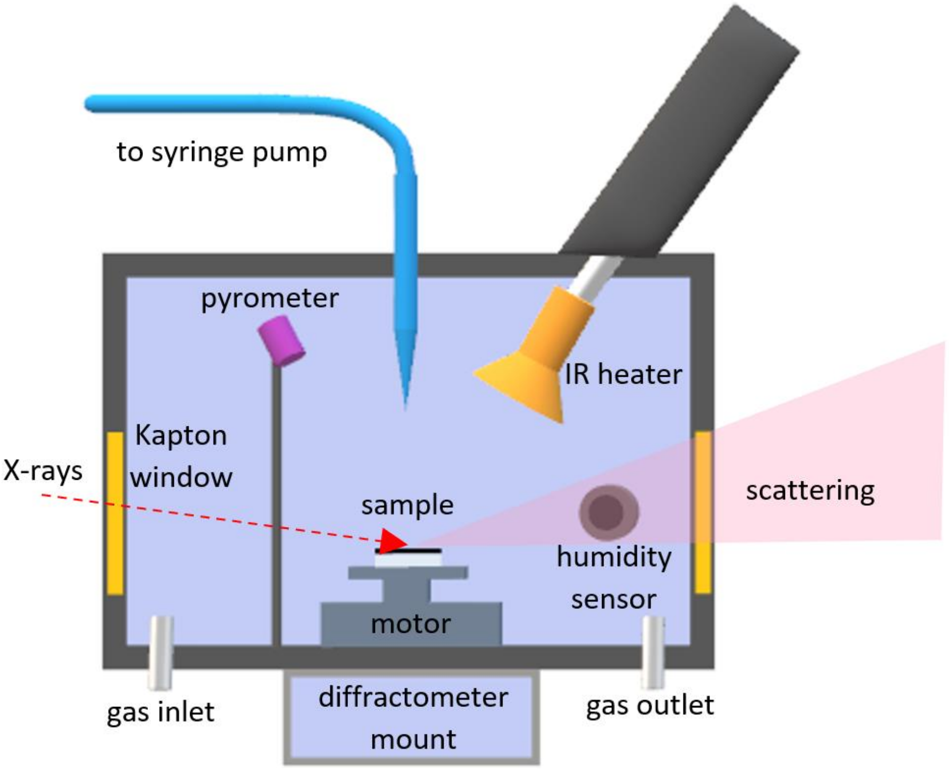


**Supplementary Figure 5** Schematic representation of the spin-coating chamber used for *in situ* GIXD measurements with $N_2$-rich atmosphere and measured humidity level. Solution deposition is being done by an automated syringe pump, sample is being annealed by an IR heater and its temperature is measured by a pyrometer.

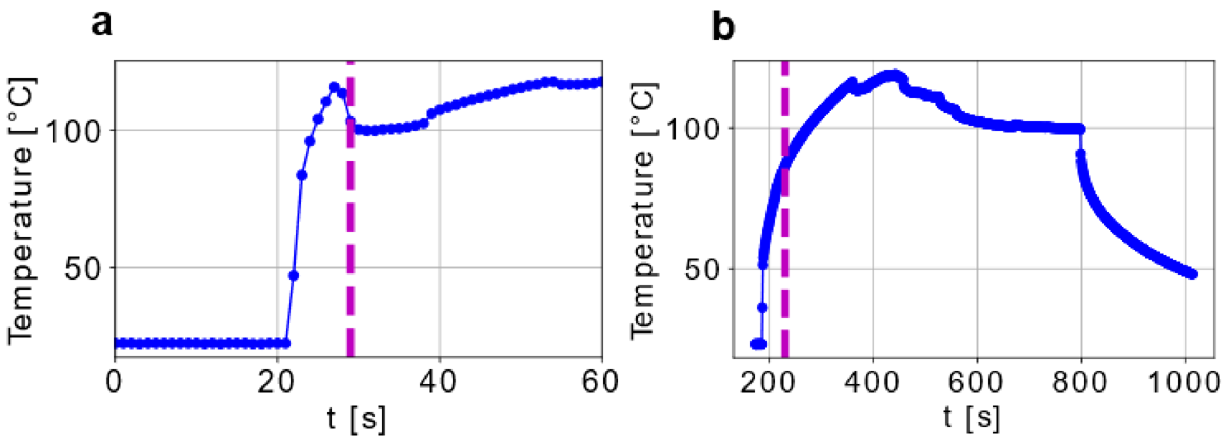


**Supplementary Figure 6** The temperature curves of the annealing processes for $(BA)_2(MA)_{n-1}Pb_nI_{3n+1}$ (**a**) and $MAPbI_3$ (**b**) measured via pyrometer. The dashed lines indicate the time of perovskite formation. The changing emissivity of the samples during the measurements can result in increased error bars for the temperature values obtained by the pyrometer.

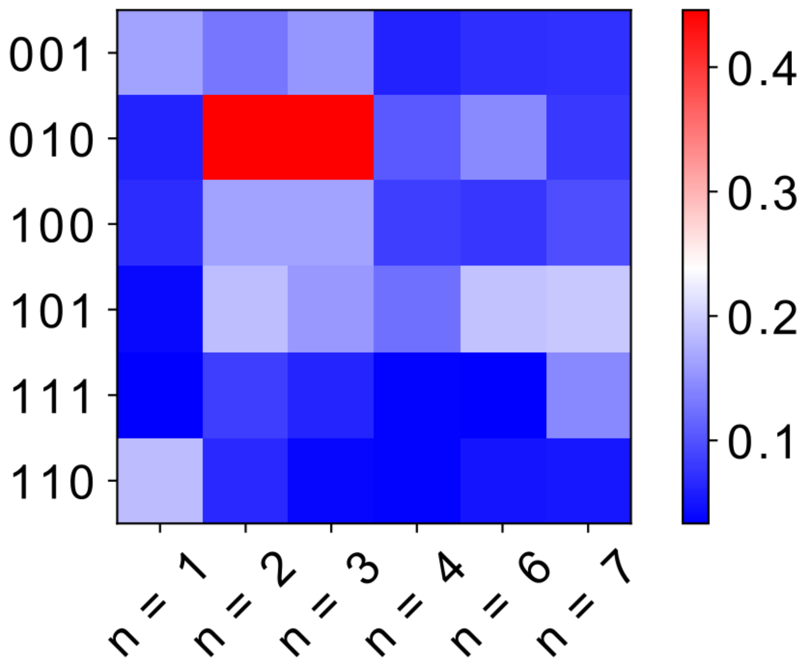


**Supplementary Figure 7** Phase matching results for the use case 1. The vertical axis corresponds for different unit cell orientations in a form of miller indices; the horizontal axis denotes different phases of $(BA)_2(MA)_{n\text{-}1}Pb_nI_{3n+1}$ 2D perovskite. The colormap shows the matching results, from which two best matches $n = 2$ and $n = 3$ with $(010)$ orientation are chosen.

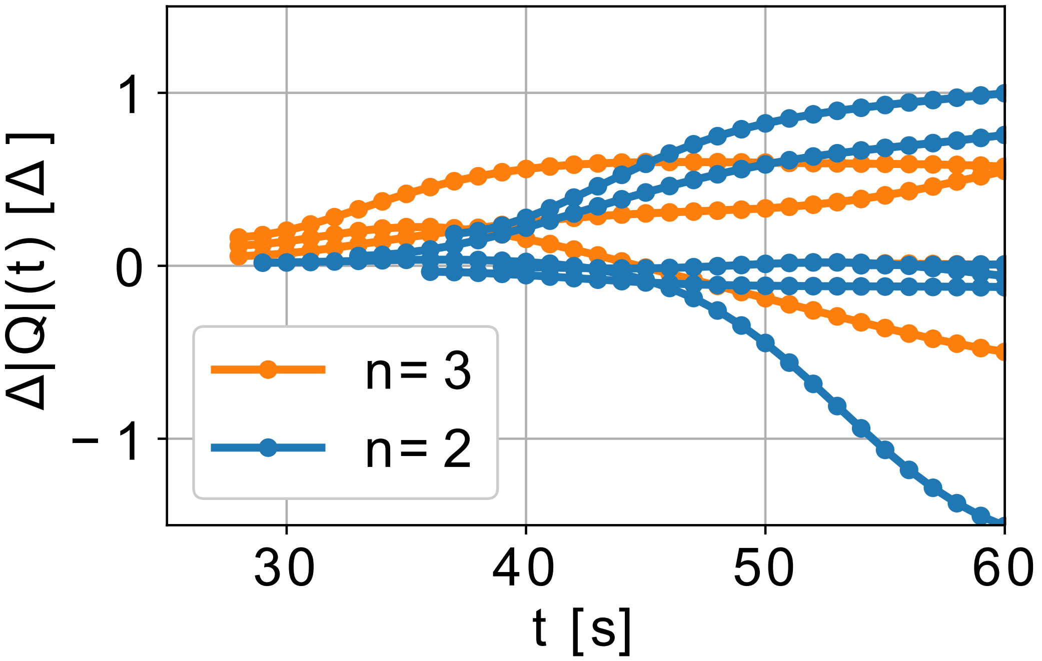


**Supplementary Figure 8** The relative peak positions for $n = 2$ and $n = 3$ phases of $(BA)_2(MA)_{n\text{-}1}Pb_nI_{3n+1}$ perovskite over time for the use case 1 calculated as $\frac{|Q|(t)}{|Q|(t_0)} - 1$.

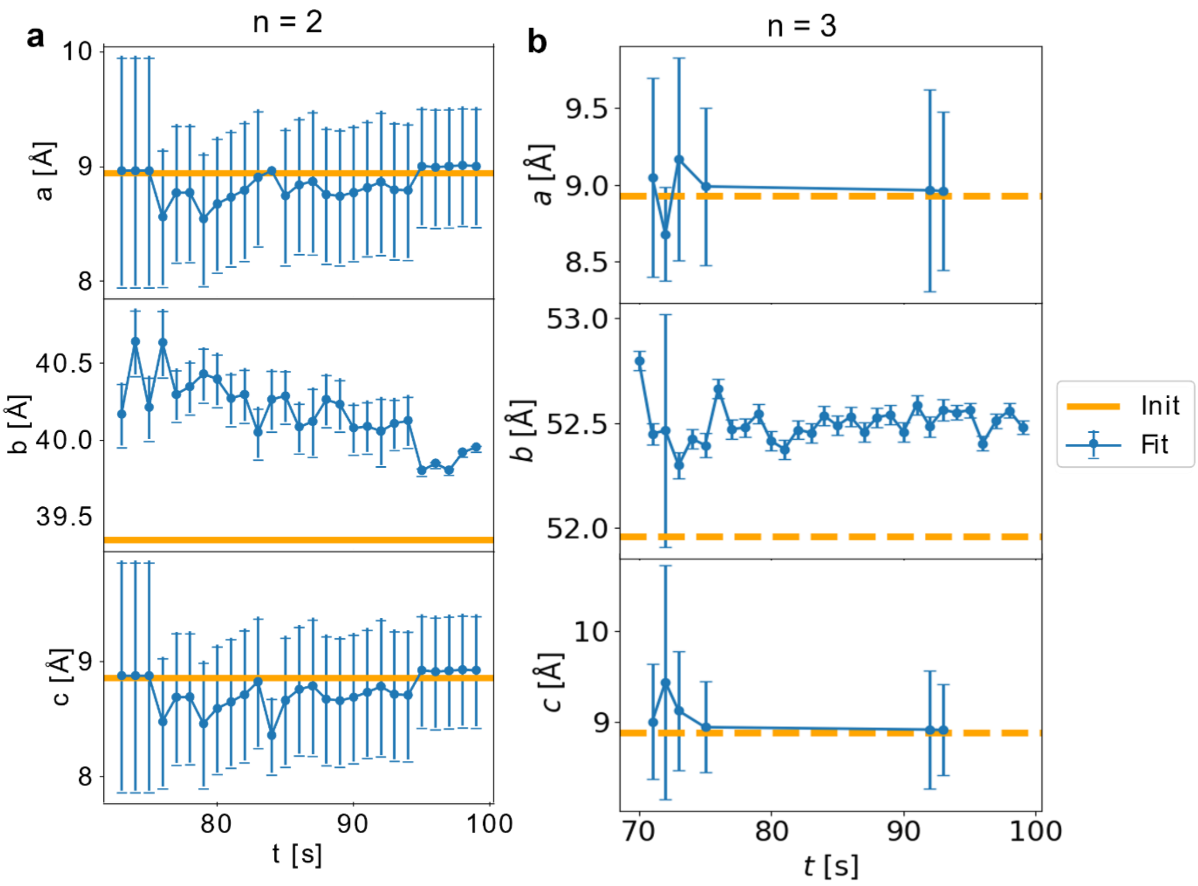


**Supplementary Figure 9** Refined lattice parameters for $n = 2$ (**a**) and $n = 3$ (**b**) phases of $(BA)_2(MA)_{n\text{-}1}Pb_nI_{3n+1}$ perovskite structures based on the positions of the detected diffraction reflections. Horizontal dash lines correspond to the initial fitting values. The missed values for $n = 3$ phase correspond to the time frames without non-overlapping in-plane detected peaks from the $n = 3$ phase with $Q_{||} \neq 0$.

| | Feature map 1 | Feature map 2 | Feature map 3 |
|---|---|---|---|
| Feature map shape | $64 \times 128$ | $32 \times 128$ | $16 \times 128$ |
| Anchor shapes | $50 \times 10$, $100 \times 10$ | $200 \times 10$, $300 \times 10$ | $400 \times 10$, $500 \times 10$ |

**Supplementary Table 1** Feature map shapes and the corresponding anchor shapes for an input image of size $512 \times 512$.

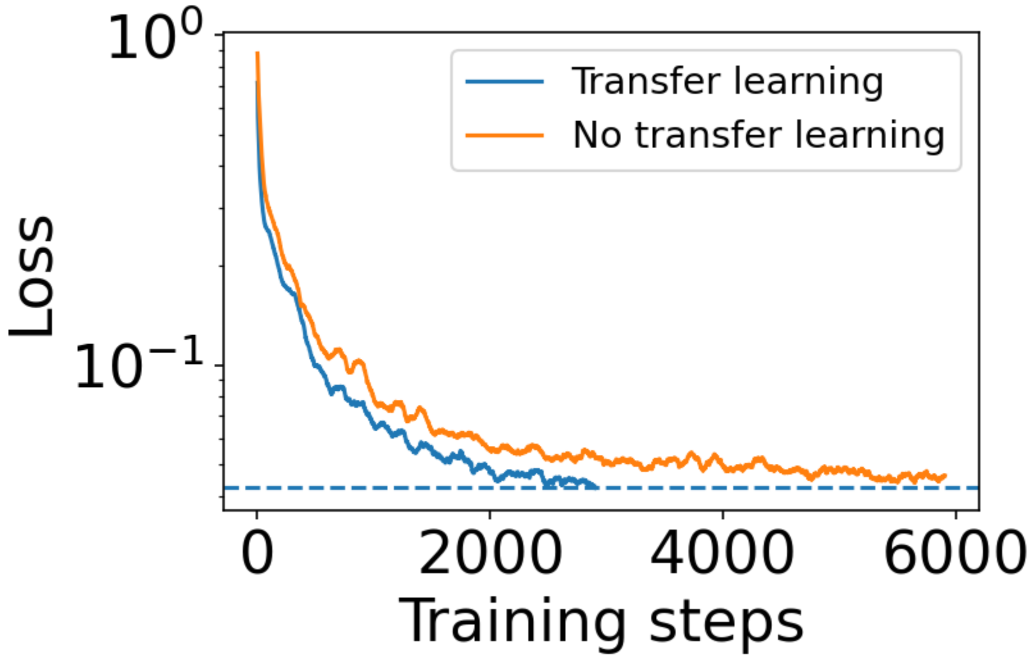


**Supplementary Figure 10** The training process for different parameter initializations. The blue curve (transfer learning) corresponds to our model initialized with the publicly available weights of the first layers of the ResNet-18 model pretrained on the classification task on ImageNet dataset. The orange curve (no transfer learning) corresponds to the standard Kaiming initialization. The transfer learning approach allows to roughly halve the training time (3000 training steps) to achieve the same performance as for the same model with the random initialization (6000 training steps).
